# Supplementary material for: Feasibility and optimum recovery in warm-start quantum optimization for a drug-response model on a trapped-ion processor
Source: arXiv:2609.22748 source file (2026-09-19)
Supplement: Supplementary file 1 [file supp_feas_rows.tex]

\newcommand{\SupplementFeasRows}{%
6 & 31.25 & 62.42 & 89.96 & 88.00 & 100.00 \\
8 & 21.88 & 40.57 & 76.26 & 73.00 & 100.00 \\
9 & 10.55 & 31.68 & 63.46 & 63.00 & 100.00 \\
10 & 11.72 & 41.37 & 77.88 & 70.50 & 100.00 \\
12 & 3.96 & 32.51 & 31.18 & 29.50 & 100.00 \\
15 & 1.10 & 34.85 & 68.70 & 65.00 & 100.00 \\
}
