# Supplementary material for: Feasibility and optimum recovery in warm-start quantum optimization for a drug-response model on a trapped-ion processor
Source: arXiv:2609.22748 source file (2026-09-19)
Supplement: Supplementary file 2 [file supp_hit_rows.tex]

\newcommand{\SupplementHitRows}{%
6 & 95.71 & 84.89 & 96.04 & 100.00 \\
8 & 54.29 & 93.63 & 99.21 & 97.28 \\
9 & 32.36 & 10.42 & 16.94 & 97.62 \\
10 & 17.75 & 80.45 & 94.02 & 81.24 \\
12 & 4.77 & 28.23 & 31.88 & 71.02 \\
15 & 0.61 & 25.02 & 39.01 & 42.67 \\
}
