# Supplementary material for: Feasibility and optimum recovery in warm-start quantum optimization for a drug-response model on a trapped-ion processor
Source: arXiv:2609.22748 source file (2026-09-19)
Supplement: Supplementary file 3 [file supp_larger_controls.tex]

\newcommand{\LargerControlRows}{%
18 & 675 & Ideal QAOA & 73.16 & 0.1666 & 51.0 \\
18 & 675 & Initial product & 37.37 & 0.0985 & 51.2 \\
18 & 675 & Uniform feasible & 100.00 & 0.1481 & 41.8 \\
20 & 650 & Ideal QAOA & 25.52 & 0.0239 & 39.0 \\
20 & 650 & Initial product & 27.80 & 0.0212 & 38.1 \\
20 & 650 & Uniform feasible & 100.00 & 0.1538 & 31.8 \\
21 & 1134 & Ideal QAOA & 73.44 & 0.1111 & 49.3 \\
21 & 1134 & Initial product & 39.11 & 0.0670 & 49.5 \\
21 & 1134 & Uniform feasible & 100.00 & 0.0882 & 40.3 \\
25 & 1500 & Ideal QAOA & 29.53 & 0.0242 & 42.4 \\
25 & 1500 & Initial product & 30.72 & 0.0222 & 42.0 \\
25 & 1500 & Uniform feasible & 100.00 & 0.0667 & 33.4 \\
30 & 2875 & Ideal QAOA & 33.39 & 0.0174 & 52.1 \\
30 & 2875 & Initial product & 33.64 & 0.0172 & 52.0 \\
30 & 2875 & Uniform feasible & 100.00 & 0.0348 & 43.2 \\
35 & 4900 & Ideal QAOA & 35.85 & 0.0120 & 50.3 \\
35 & 4900 & Initial product & 35.75 & 0.0122 & 50.3 \\
35 & 4900 & Uniform feasible & 100.00 & 0.0204 & 41.7 \\
}
