# Supplementary material for: Feasibility and optimum recovery in warm-start quantum optimization for a drug-response model on a trapped-ion processor
Source: arXiv:2609.22748 source file (2026-09-19)
Supplement: Supplementary file 4 [file supp_larger_hardware.tex]

\newcommand{\LargerHardwareRows}{%
18 & 07-11 06:06 & 42.0 & 0.0 & 48.9 \\
18 & 07-11 07:55 & 49.5 & 0.5 & 47.1 \\
18 & 07-12 13:37 & 46.0 & 0.5 & 50.0 \\
20 & 07-11 08:09 & 20.0 & 0.0 & 37.7 \\
20 & 07-12 13:47 & 27.0 & 0.0 & 37.7 \\
21 & 07-11 06:09 & 44.0 & 0.5 & 49.0 \\
21 & 07-11 08:02 & 40.5 & 0.0 & 47.4 \\
21 & 07-12 13:40 & 35.0 & 0.0 & 47.8 \\
25 & 07-11 08:17 & 13.0 & 0.0 & 39.3 \\
25 & 07-12 13:54 & 15.0 & 0.0 & 38.6 \\
30 & 07-11 08:23 & 6.5 & 0.0 & 43.1 \\
35 & 07-11 08:33 & 3.5 & 0.0 & 47.5 \\
}
