# Supplementary material for: Feasibility and optimum recovery in warm-start quantum optimization for a drug-response model on a trapped-ion processor
Source: arXiv:2609.22748 source file (2026-09-19)
Supplement: Supplementary file 5 [file supp_panel_rows.tex]

\newcommand{\PanelRows}{
1 & 0 & 64.00 & 2.682 & 1.265 & 0.617\\
1 & 1 & 61.68 & 2.230 & 1.265 & 0.617\\
1 & 2 & 64.75 & 2.752 & 1.265 & 0.617\\
2 & 0 & 63.42 & 3.365 & 1.485 & 0.617\\
2 & 1 & 62.65 & 3.319 & 1.485 & 0.617\\
2 & 2 & 63.91 & 3.427 & 1.485 & 0.617\\
3 & 0 & 64.89 & 3.279 & 1.436 & 0.617\\
3 & 1 & 64.31 & 3.248 & 1.436 & 0.617\\
3 & 2 & 64.05 & 3.219 & 1.436 & 0.617\\
4 & 0 & 66.51 & 2.894 & 1.295 & 0.617\\
4 & 1 & 65.66 & 2.809 & 1.295 & 0.617\\
4 & 2 & 66.05 & 2.865 & 1.295 & 0.617\\
}
