# Supplementary material for: Feasibility and optimum recovery in warm-start quantum optimization for a drug-response model on a trapped-ion processor
Source: arXiv:2609.22748 source file (2026-09-19)
Supplement: Supplementary file 6 [file supp_recovered_quality.tex]

\newcommand{\RecoveredQualityRows}{%
6 & 2 & 07-03 03:33 & 442 & 35.2 & 0.0 & 21\\
6 & 2 & 07-03 05:16 & 176 & 33.5 & 0.0 & 21\\
6 & 2 & 07-11 07:10 & 171 & 35.5 & 0.0 & 21\\
8 & 2 & 07-03 05:25 & 146 & 38.3 & 0.0 & 37\\
8 & 2 & 07-11 07:12 & 144 & 36.2 & 0.0 & 37\\
9 & 3 & 07-03 05:33 & 126 & 33.5 & 22.1 & 33\\
10 & 2 & 07-03 05:41 & 141 & 38.3 & 30.3 & 53\\
10 & 2 & 07-11 07:19 & 139 & 40.4 & 0.0 & 53\\
12 & 2 & 07-11 07:25 & 145 & 53.1 & 0.0 & 69\\
12 & 3 & 07-03 05:51 & 59 & 34.5 & 39.5 & 57\\
14 & 2 & 07-11 07:38 & 124 & 50.0 & 0.0 & 85\\
15 & 3 & 07-03 06:03 & 130 & 39.7 & 18.8 & 81\\
15 & 3 & 07-11 07:48 & 109 & 40.1 & 16.2 & 81\\
18 & 3 & 07-11 06:06 & 84 & 48.9 & 12.5 & 105\\
18 & 3 & 07-11 07:55 & 99 & 47.1 & 0.0 & 105\\
18 & 3 & 07-12 13:37 & 92 & 50.0 & 0.0 & 105\\
20 & 5 & 07-11 08:09 & 40 & 37.7 & 27.9 & 97\\
20 & 5 & 07-12 13:47 & 54 & 37.7 & 27.9 & 97\\
21 & 3 & 07-11 06:09 & 88 & 49.0 & 0.0 & 129\\
21 & 3 & 07-11 08:02 & 81 & 47.4 & 26.3 & 129\\
21 & 3 & 07-12 13:40 & 70 & 47.8 & 26.7 & 129\\
25 & 5 & 07-11 08:17 & 26 & 39.3 & 9.1 & 137\\
25 & 5 & 07-12 13:54 & 30 & 38.6 & 20.5 & 137\\
30 & 5 & 07-11 08:23 & 13 & 43.1 & 35.0 & 177\\
35 & 5 & 07-11 08:33 & 7 & 47.5 & 40.4 & 200\\
}
